# Supplementary material for: Bacterial diffusion in disordered media, by forgetting the media
Source: arXiv:2311.10612 ancillary file (2023-12-27)
Supplement: Supplementary file 1 [file SI_v2.pdf]

# Supporting Information for: Bacterial diffusion in disordered media, by forgetting the media

Henry H. Mattingly[1, *]

[1] *Center for Computational Biology, Flatiron Institute, Simons Foundation*

(Dated: November 17, 2023)

## ENVIRONMENT STATISTICS

First, we derive some useful properties of the Poisson obstacle environment considered here. The circular obstacles are placed independently of each other, with the positions of their centers generated by a Poisson point process in two dimensions. The key parameter of this process is the number density of obstacles $\rho$, which is the average number of points (obstacle centers) per unit area. For finite-sized obstacles, a second important parameter is the reduced density $\eta = \rho\ A_0$, where $A_0$ is the area of the obstacle [1]. For circular obstacles of radius $R = 1$, $A_0 = \pi$ and $\eta = \pi\ \rho$. Furthermore, the number of circles whose centers all located inside an area $A_0$ is Poisson-distributed with mean $\eta$.

### Void volume fraction

The volume fraction of void space is the probability that no obstacles overlap a given point. This is equivalent to the probability that no circles have their centers inside an area $A_0$ centered on the given point [1]. From the Poisson distribution, this is

$$\phi_{\text{void}} = \exp(-\eta) = \exp(-\pi\ \rho). \tag{1}$$

### Obstacle encounter rate from void space

The Poisson properties of the environment can also be used to derive the chord length distribution, which is the distribution of lengths of straight line segments that lie entirely in the void space, starting and ending at obstacle surfaces. For obstacles generated by a Poisson process, this is equivalent to the segment-length distribution [2], which is the distribution of lengths of straight rays that start at a random point in the void space and end at the first obstacle encountered.

The survival probability of a line segment, $S(L)$, is the probability that no obstacle intersects a segment of length $L$. This quantity is exactly the same as the lineal-path function defined by Torquato and colleagues [2–4]. For circular obstacles, this is the probability that no obstacle center lies inside a region consisting of a rectangle with semicircular caps at each end, centered on the line segment (Fig. 1A). The area of this region is $A = 2L + \pi$.

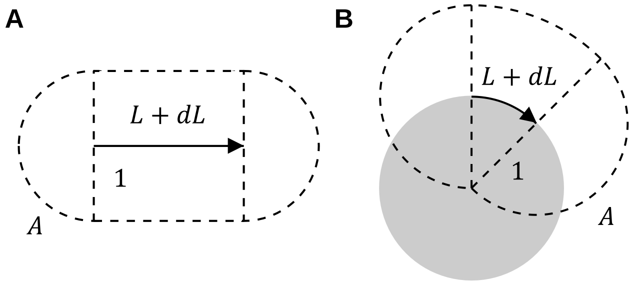


FIG. 1. Obstacle encounter rate derivations. A) The obstacle encounter rate in state 0, and the mean chord length, can be derived from the probability that no obstacles lie in area A, delimited by the dashed lines. B) The obstacle encounter rate in state 1 can be derived in a similar way, using the probability that no obstacles lie in the area delimited by the dashed lines.

Thus, $S_0(L) = \exp(-\rho\ A) = \exp(-\rho\ (2L+\pi))$, with subscript 0 to indicate that the line lies in the void space.

As the length of the line segment increases, the rate at which an obstacle is encountered can be determined from standard hazard analysis. This is $h_0(L) = -\mathrm{d}\log(S_0(L))/\mathrm{d}L = 2\rho$ (ref). Furthermore, the chord-length and line-segment distributions are exponential:

$$p_0(L) = 2\rho\ \exp(-2\rho\ L), \tag{2}$$

with mean chord length

$$\gamma = (2\ \rho)^{-1}, \tag{3}$$

The obstacle encounter rate per unit length can be written:

$$h_0 = \gamma^{-1}. \tag{4}$$

### Second obstacle encounter rate

We can also derive the rate at which a second circle is encountered as one follows the perimeter of a first circle. For this, we need the survival probability of a curve of length $L$ on a circle of radius $R$. For no obstacles to intersect the curve, there must be no obstacle centers inside a pie slice (or "sector") of angle $\theta$ out of a circle of radius $2R$ that is centered on the circular obstacle, along with two semicircular caps (Fig. 1B). The area of this region is $A = (2R)^2\ \theta/2 + \pi\ R^2 = 2\ \theta + \pi$ (using

$R = 1$). The arc length $L$ of the curve on the obstacle is $L = R\,\theta = \theta$. Thus, the survival probability of the curve is $S_1(L) = \exp(-\rho\,(2L + \pi))$, and the obstacle encounter rate per unit length is

$$h_1 = 2\;\rho = \gamma^{-1}. \tag{5}$$

### Distribution of distances between the centers of two overlapping circles

Given that two circles overlap, we can derive the distribution of the distance between their centers, which will be useful below. To overlap, the distance $r$ between their centers must lie in $r \in [0, 2]$. Fixing the location of the first circle, the center of the second circle can lie anywhere on the perimeter of a circle of radius $r$ centered on the first one. Thus, the number of ways that the second circle can be placed increases linearly with $r$. Since obstacle centers are uniformly distributed, this means

$$p(r) = r/2, \quad r \in [0, 2], \tag{6}$$

where the factor of 1/2 comes from normalization.

### Distribution of nearest neighbor distances of the Poisson process

Finally, one can also derive the distribution of the distance from one point of the Poisson process to its nearest neighbor. The survival probability of no circles having their centers within a distance $r$ of a given point is $S_{nn}(r) = \exp(-\rho\;\pi\;r^2)$. The encounter rate with a center is then $h_{nn}(r) = 2\pi\rho\;r$. The distribution of nearest neighbor distances is $p_{nn}(r) = h(r)\exp(-\int_0^r h(r')\;\mathrm{d}r')$, or

$$p_{nn}(r) = 2\pi\rho\;r\;\;\exp(-\pi\rho\;r^2). \tag{7}$$

## SLIDING ON AN OBSTACLE SURFACE

### Sliding dynamics

When the cell is pushing against one obstacle, its velocity can be written from the balance of a propulsion force, a drag force, and a force from the hard obstacle as:

$$\boldsymbol{v}(t) = \hat{\boldsymbol{u}}(t) - \alpha(t)\;\boldsymbol{n}(t), \tag{8}$$

where $\boldsymbol{n}(t)$ is the inward surface normal. To compute $\nu$, we will need $\boldsymbol{v}(t) \cdot \hat{\boldsymbol{u}}(t)$. Furthermore, to compute the average rate at which the cell encounters a second obstacle when in state 1, we will need the average of its surface tangential speed, $|\boldsymbol{v}(t)|$.

The projection of cell's velocity onto the surface normal of the obstacle must be zero, $\boldsymbol{v} \cdot \boldsymbol{n}(t) = 0$, giving

$$\alpha(t) = \hat{\boldsymbol{u}}(t) \cdot \boldsymbol{n}(t). \tag{9}$$

The cell's velocity thus only has a component tangential to the obstacle surface,

$$\boldsymbol{v}(t) = \sqrt{1 - \alpha(t)^2}\;\boldsymbol{t}(t), \tag{10}$$

where $\boldsymbol{t}(t)$ is the surface tangent vector, chosen so that $\boldsymbol{t}(t) \cdot \hat{\boldsymbol{u}}(t) \geq 0$. The projection of the cell's velocity onto its heading is

$$\boldsymbol{v}(t) \cdot \hat{\boldsymbol{u}}(t) = 1 - \alpha(t)^2. \tag{11}$$

Next we define $\theta(t)$ to be the angle between the cell's heading $\hat{\boldsymbol{u}}(t)$ and the inward pointing surface normal $\boldsymbol{n}(t)$ (Fig. 2), so that $\cos(\theta(t)) = \alpha(t)$. As the cell slides along the surface of the obstacle, the dynamics of this angle are:

$$\dot{\theta}(t) = \sin(\theta(t)), \quad \theta(0) = \theta_0, \tag{12}$$

with initial encounter angle $\theta_0$ (see also [5, 6]). The solution to this ODE is:

$$\begin{aligned} \theta(t) &= 2\cot^{-1}\left(e^{-t}\cot(\theta_0/2)\right), \quad t \in [0, t_{\mathrm{esc}}(\theta_0)] \\ t_{\mathrm{esc}}(\theta_0) &= \log\left(\cot(\theta_0/2)\right), \end{aligned} \tag{13}$$

where the time at which the cell escapes from state 1 by sliding off the obstacle, $t_{\mathrm{esc}}(\theta_0)$, is the time when the cell's heading is perpendicular to the surface normal, or $\theta(t_{\mathrm{esc}}) = \pi/2$, and it depends on the initial encounter angle $\theta_0$.

### Distribution of surface angles

To compute several parameters of the Markov model, we will need the distribution of $\theta$, the cell heading on an obstacle surface relative to the surface normal vector. The dynamics of the "surface angle" $\theta$ can be included as another dependent variable in state 1 of the three-state Markov. However, to reduce clutter, we treat it here separately.

Deriving this distribution is challenging, even in simpler geometries [7]. Therefore, we will make several simplifying assumptions. First, we assume that the distribution has reached steady state, which is an assumption we'll make anyway during the homogenization procedure. Next, anticipating that the dynamics in state 1 will be important only for cells with long run lengths, we neglect tumbles in this derivation of the distribution of $\theta$. Next, we assume that the flux into state 1 is dominated by cells arriving from state 0, which are uniformly distributed in space and heading. This assumption determines the distribution of initial angles $\theta_0$ arriving at the surface. Due

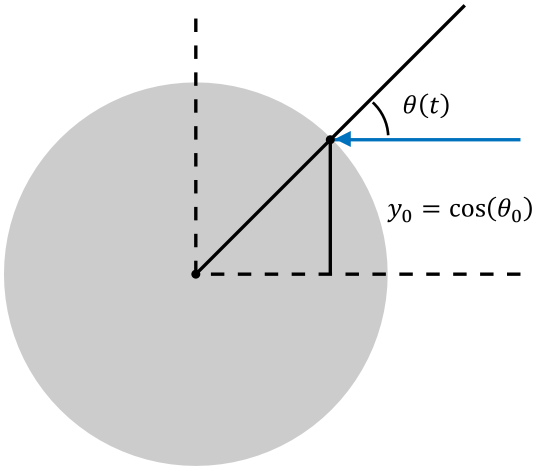


FIG. 2. Deriving the distribution of cell surface headings relative to the surface normal, $\theta$, in state 1. Cells encounter obstacles with initial angle $\theta_0$ between its heading and the outward surface normal, which then evolves in time as the cell slides on the surface, $\theta(t)$. $y_0$ is the vertical position of the cell relative to the center of the obstacle at the initial point of contact. Using obstacle symmetry, and assuming cell positions and headings in the bulk are uniformly distributed, then $y_0$ is uniformly distributed between 0 and 1, so $p(\theta_0) = \cos(\theta_0)$. The blue arrow represents the cell's heading vector, $\hat{\boldsymbol{u}}$. If the cell reaches a surface heading (or position) of $\theta(t) = \pi/2$, it slides off the surface and back into the bulk.

to obstacle symmetry, we can focus on cells arriving with heading $\hat{\boldsymbol{u}} = (-1, 0)$ at a circle centered at the origin. For uniformly distributed positions in the bulk, the cells arrive at the surface with vertical position $y_0 = \sin(\theta_0)$ uniformly distributed between 0 and 1. Thus, the relative arrival flux at angle $\theta_0$ is proportional to $\cos(\theta_0)$. This assumption is expected to break down when the cells are strongly confined by obstacles, $\gamma <\sim 1$ [7].

With these assumptions, we can write down a differential equation for the dynamics of $p(\theta, \theta_0)$, the joint distribution of initial and instantaneous cell headings:

$$\partial_\theta \left(\sin(\theta)\ p(\theta, \theta_0)\right) = \frac{\cos(\theta_0)}{Z}\delta(\theta - \theta_0) - h_1 \sin(\theta)\ p(\theta, \theta_0), \quad \theta, \theta_0 \in [0,\ \pi/2]. \tag{14}$$

The left-hand side accounts for sliding on the obstacle surface (Eqn. 12). The first term on the right-hand side is the flux of arriving cells, using the encounter rate per unit angle (or arc length) from Eqn. 5. $Z$ is a constant that will be determined by normalization. The last term is the loss of cells that encounter a second obstacle. Most of these cells enter state 2. Those that continue sliding on another obstacle technically count as an additional arrival flux at some initial angle $\theta_0$ between the cell's heading and the surface normal of the new obstacle. However, that flux is small compared to arrivals from the bulk, so we ignore it. The "initial condition" on $\theta$ is already accounted for by the incoming flux term, so we drop the constant of integration when solving this ODE.

Solving the ODE for $p(\theta, \theta_0)$ gives:

$$p(\theta, \theta_0) = \frac{\cos(\theta_0)}{Z\sin(\theta)} \exp\left(-\gamma^{-1}(\theta - \theta_0)\right)\ \Theta(\theta - \theta_0), \tag{15}$$

where $\Theta(x)$ is the Heaviside step function. The exponential term is essentially the probability of not hitting a second obstacle between angles $\theta_0$ and and $\theta$. Integrating over initial angles $\theta_0$ gives the distribution of surface angles $\theta$:

$$p(\theta) = \frac{1}{Z}\frac{1 + \gamma^{-1}(\cot(\theta) + \csc(\theta)\exp(-\gamma^{-1}\theta))}{1 + \gamma^{-2}}, \tag{16}$$

and $Z$ is given by normalization: $\int_0^{\pi/2} p(\theta)\mathrm{d}\theta = 1$. In the regime of dilute obstacles, $\gamma \gg 1$,

$$Z \approx \pi/2 - \ln(2)\ \gamma^{-1}. \tag{17}$$

Note that theoretical curves in the main text were generated *without* using the dilute obstacle approximation.

## Average projected speed in state 1

In the Markov model, we will neglect displacements of the cell perpendicular to its heading $\hat{\boldsymbol{u}}$ because they have small effects on the diffusion coefficient when the obstacles are circular and randomly placed (see also [6]). This is because either the obstacle radius is small compared to the run length, $\beta \ll 1$, and therefore perpendicular displacements are small; or the obstacle radius is large compared to the run length, $\beta \gg 1$, and the cell tumbles before the perpendicular displacement is significant.

The cell's average speed in state 1 projected onto its heading $\hat{\boldsymbol{u}}$ is:

$$\begin{aligned} \nu &= \langle \boldsymbol{v}(t) \cdot \hat{\boldsymbol{u}}(t) \rangle \\ &= \int_0^{\pi/2} \sin^2(\theta)\ p(\theta)\mathrm{d}\theta \\ &= \frac{1}{Z\ (1 + \gamma^{-2})}\left(\frac{\pi}{4} + \gamma^{-1}\left(\frac{1}{2} - \frac{1 - \gamma^{-1}\exp(-\frac{\pi}{2}\gamma^{-1})}{1 + \gamma^{-2}}\right)\right). \end{aligned} \tag{18}$$

In the dilute regime, $\gamma \gg 1$, this is approximately

$$\nu \approx \frac{1}{2} - \gamma^{-1}\ \pi^{-1}(1 - \ln(2)). \tag{19}$$

## Slide-off transition rate from state 1 to state 0

Since $p(\theta)$ is normalized, the rate at which cells slide off of an obstacle is given by the flux at $\theta = \pi/2$. Since the flux is $\sin(\theta)\ p(\theta)$, we use Eqn. 16 to get:

$$k_{10} = \frac{1}{Z}\frac{1 - \gamma^{-1}\exp(-\frac{\pi}{2}\gamma^{-1})}{1 + \gamma^{-2}}. \tag{20}$$

In the dilute regime $\gamma \gg 1$, this is approximately

$$k_{10} \approx \frac{2}{\pi} - \gamma^{-1}\left(\frac{2}{\pi} - \frac{\ln(16)}{\pi^2}\right). \tag{21}$$

### Transition rate from state 1 to state 2

Since $p(\theta)$ is normalized, the total rate at which cells in state 1 encounter a second obstacle is the integral of the encounter term in Eqn. 14, over all angles $\theta_0$ and $\theta$. Technically, not all of the cells that encounter a second obstacle transition to state 2: some arrangements of cell headings and obstacle positions cause the cell to continue sliding on the second obstacle, thus remaining in state 1. However, most encounters ($\sim 90\%$ in simuations) lead to a transition to state 2. Therefore, we make the approximation that all cells transition to state 2 upon encounter with a second obstacle, which upper bounds the actual transition rate. With this,

$$\begin{aligned} k_{12} &= \gamma^{-1}\int_0^{\pi/2} \sin(\theta)\ p(\theta)\mathrm{d}\theta \\ &= \gamma^{-1}\frac{1}{Z}\frac{\gamma^{-1} + \exp(-\frac{\pi}{2}\gamma^{-1})}{1+\gamma^{-2}}. \end{aligned} \tag{22}$$

Note that this is the same as the average speed of the cell tangential to the obstacle surface, multiplied by $\gamma^{-1}$. In the regime of dilute obstacles $\gamma \gg 1$, this is approximately

$$k_{12} \approx \gamma^{-1}\frac{2}{\pi} - \gamma^{-2}\left(1 - \frac{2}{\pi}\left(1 + \pi^{-1}\ln(4)\right)\right). \tag{23}$$

## REMAINING TRANSITION RATES

### Transition rate from state 0 to state 1

The transition from state 0, in the void space, to state 1, on the surface of one obstacle occurs with rate $k_{01}$. This is just the cell's swimming speed (rescaled to 1), times the obstacle encounter rate per unit length, $h_0$ (Eqn. 4):

$$k_{01} = \gamma^{-1}. \tag{24}$$

### Transitions due to tumbles

What remains is to compute the probability that a tumble in one state leads to transition to another state. Tumbles occur at rate $\beta^{-1}$, but a tumble does not always lead to a state transition. In state 0, tumbles always keep the cell in state 0.

In state 1, tumbles can lead to a transition to state 0. This is especially simple because the obstacles are convex and rotationally symmetric. Any post-tumble heading $\hat{\boldsymbol{u}}$ that has a component pointing into an obstacle surface remains in state 1. Tumbles fully reorient, and half of all possible headings point out of the obstacle surface. Therefore, the probability that a tumble in state 1 transitions the cell to state 0 is:

$$p_{10} = 1 - p_{11} = 1/2. \tag{25}$$

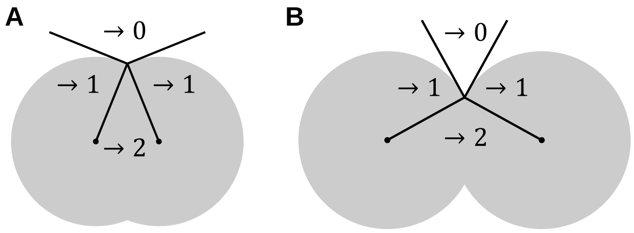


FIG. 3. Examples of configurations of pairs of obstacles that can trap a cell at their intersection. In a given configuration, if a trapped cell tumbles, then the sector in which its post-tumble heading lies determines which state it will be in after the tumble. For obstacle pairs whose centers are closer to other (smaller $r$), as in (A), the probability that a tumble transitions to state 0 is higher, indicated by the larger width of the sector labeled 0. For obstacle pairs whose centers are further apart (larger $r$), as in (B), the cell is more likely to remain in state 2. The probabilities $p_{2j}$ of transitioning from state 2 to state $j$ result from an average over these configurations.

Transitions out of state 2 due to tumbles are more complicated. The probability that a tumble leads to a state transition depends on the configuration of the two obstacles that trap the cell (Fig. 3). The obstacle configuration is fully specified by the distance between the obstacle centers, $r$. For a given $r$, we can determine the probability of each transition.

For two obstacles of radii $R = 1$ to be in contact with each other, the distance between their centers, $r$, must be in $r \in [0, 2]$. Due to symmetry, suppose that the first circle's center is located at the origin, and the second circle's center is located on the $x$-axis at position $(r, 0)$. The two circles intersect at points $(r/2, \pm\sqrt{1-(r/2)^2}$. Taking the positive intersection, the intersection point is located on the first circle at angle $\theta_r(r)$ with the $x$-axis:

$$\theta_r(r) = \arctan\left(\frac{\sqrt{1-(r/2)^2}}{r/2}\right). \tag{26}$$

For the cell to remain trapped after the tumble, its heading must lie within the minor sector formed by the inward-pointing normals of the two obstacles, at their point of intersection (the region marked "$\rightarrow$ 2" in Fig. 3AB). The angle between these normal vectors is:

$$\theta_n(r) = \pi - 2\ \theta_r(r). \tag{27}$$

Thus, any post-tumble heading relative to the first obstacle's normal vector that lies in $\theta \in [0, \theta_n(r)]$ will remain in state 2. Since tumbles fully reorient, the probabiltiy that the cell remains in state 2, for a given $r$, is:

$$p_{22}(r) = \frac{\theta_n(r)}{2\pi} = \frac{1}{2} - \frac{\theta_r(r)}{\pi}. \tag{28}$$

For the cell to transition to state 1 after a tumble, its heading must lie between the surface normal and tangent vectors of one of the two obstacles. This angle must be $\pi/2$. Since tumbles fully reorient, and since there are two regions of angle $\pi/2$ that lead to transition to state 1, we have:

$$p_{21}(r) = \frac{\pi}{2\pi} = 1/2, \tag{29}$$

which is independent of $r$.

For a given $r$, a tumble transition the cell to state 0 if the post-tumble heading lies between the two surface tangent vectors that point out of the intersection point. But since tumbles must leave the cell in one of the two configurations, this is simply given by

$$p_{20}(r) = 1 - p_{21} - p_{22} = \frac{\theta_r(r)}{\pi}. \tag{30}$$

Finally, we need to average these transition probabilities over distances $r$ between obstacle centers. Using Eqn. 6:

$$\begin{aligned} p_{20} &= \int_0^{\pi/2} p_{20}(r)\ p(r)\mathrm{d}r = 1/4 \\ p_{21} &= \int_0^{\pi/2} p_{21}(r)\ p(r)\mathrm{d}r = 1/2 \\ p_{22} &= \int_0^{\pi/2} p_{22}(r)\ p(r)\mathrm{d}r = 1/4 \end{aligned} \tag{31}$$

These are the expressions used in the main text. However, they are technically incorrect. For one thing, the distribution of center-center distances $r$ in which cells get trapped is biased–it is not $p(r)$ in Eqn. 6. In the section **Transition rate from state 1 to state 2**, we neglected the possibility that encountering a second obstacle did not lead to trapping. If we had taken this into account, then the probability that an encounter leads to trapping depends on $r$. In other words, some values of $r$ are more likely to trap cells than others, and therefore this selects on the distribution of $r$. Because we neglect this effect, we overestimate $p_{20}$ and underestimate $p_{22}$. Since $p_{21}$ does not depend on $r$, it is unaffected by this bias.

Furthermore, on top of the distribution of $r$ in which cells are trapped, there is an additional source of bias that affects the parameters $p_{20}$ and $p_{22}$. For larger $r$, the probability that a tumble remains in state 2, $p_{22}(r)$ is larger. Therefore, there is a larger chance that after the tumble, the cell is still trapped. Thus, traps with larger $r$ require more tumbles on average to escape from, which should give them additional weight.

To compute this bias, given $r$, the number of tumbles until escape is given by a geometric distribution with probability of success $q = 1 - p_{22}(r)$. The average number of trials to success is $\langle N \rangle = 1/q = 1/(1 - p_{22}(r))$. Therefore, $p(r)$ in the integrals in Eqns. 31 should be multiplied by $1/(1 - p_{22}(r))$ and renormalized. By ignoring this effect for simplicity, we further overestimate $p_{20}$ and underestimate $p_{22}$.

All together, $p_{20} \sim 0.18$ and $p_{22} \sim 0.32$ in simulations, rather than 1/4 each as given in Eqn. 31.

## DIFFUSION EQUATION

In this section, we derive a long-time diffusion equation from the Markovian state model using homogenization techniques. The partial differential equations of the Markov model in the main text are:

$$\begin{aligned} \partial_t \psi_0(\boldsymbol{x}, t, \hat{\boldsymbol{u}}) + \nabla_x \cdot (\hat{\boldsymbol{u}}\ \psi_0) &= -\left(\beta^{-1} + k_{01}\right) \psi_0 + k_{10}\ \psi_1 + \frac{\beta^{-1}}{2\pi}(P_0 + p_{10}\ P_1 + p_{20}\ P_2) \\ \partial_t \psi_1(\boldsymbol{x}, t, \hat{\boldsymbol{u}}) + \nu\ \nabla_x \cdot (\hat{\boldsymbol{u}}\ \psi_1) &= -\left(\beta^{-1} + k_{10} + k_{12}\right) \psi_1 + k_{01}\ \psi_0 + \frac{\beta^{-1}}{2\pi}\ (p_{11}\ P_1 + p_{21}\ P_2) \\ \partial_t \psi_2(\boldsymbol{x}, t, \hat{\boldsymbol{u}}) &= -\beta^{-1}\ \psi_2 + k_{12}\ \psi_1 + \frac{\beta^{-1}}{2\pi}\ p_{22}\ P_2. \end{aligned} \tag{32}$$

Here, $\psi_i(\boldsymbol{x}, t, \hat{\boldsymbol{u}})$ is the probability density of cells located at position $\boldsymbol{x}$, with heading $\hat{\boldsymbol{u}}$, at time $t$, in state $i$. $P_i(\boldsymbol{x}, t) = \int \psi_i(\boldsymbol{x}, t, \hat{\boldsymbol{u}})\ \mathrm{d}\hat{\boldsymbol{u}}$ is the marginal density of cells.

To derive the long-time and -length scale behavior of this model, we take an approach similar to that of ref [8] (see also [9–13]). Anticipating diffusive behavior, we introduce slow time $\tau = \epsilon^2\ t$ and long lengths $\boldsymbol{\xi} = \epsilon\ \boldsymbol{x}$, where $\epsilon \ll 1$ is a small parameter. Next, we write the distribution functions $\psi_i$ as an asymptotic power series

in $\epsilon$:

$$\psi_i(\boldsymbol{\xi}, t, \hat{\boldsymbol{u}}) \approx \psi_i^{(0)} + \epsilon\ \psi_i^{(1)} + \epsilon^2\ \psi_i^{(2)} + \mathcal{O}(\epsilon^3) \tag{33}$$

where subscripts still refer to the state, and superscripts in parentheses refer to the order of $\epsilon$ in the expansion.

Plugging this approximation into Eqn. 32, with long space and time variables, we get terms of varying order in $\epsilon$. In particular, note that time derivatives are multiplied by $\epsilon^2$, and spatial derivatives are multiplied by $\epsilon$. Next, we collect terms at each order of $\epsilon$, giving three sets of equations. To see what we need to compute to get a diffusion coefficient, we jump straight to the second-order equations:

$$\begin{aligned}
\partial_\tau \psi_0^{(0)}(\boldsymbol{\xi}, \tau, \hat{\boldsymbol{u}}) + \nabla_\xi \cdot (\hat{\boldsymbol{u}}\ \psi_0^{(1)}) &= -\left(\beta^{-1} + k_{01}\right) \psi_0^{(2)} + k_{10}\ \psi_1^{(2)} + \frac{\beta^{-1}}{2\pi} \left(P_0^{(2)} + p_{10}\ P_1^{(2)} + p_{20}\ P_2^{(2)}\right) \\
\partial_\tau \psi_1^{(0)}(\boldsymbol{\xi}, \tau, \hat{\boldsymbol{u}}) + \nu\ \nabla_\xi \cdot (\hat{\boldsymbol{u}}\ \psi_1^{(1)}) &= -\left(\beta^{-1} + k_{10} + k_{12}\right) \psi_1^{(2)} + k_{01}\ \psi_0^{(2)} + \frac{\beta^{-1}}{2\pi} \left(p_{11}\ P_1^{(2)} + p_{21}\ P_2^{(2)}\right) \\
\partial_\tau \psi_2^{(0)}(\boldsymbol{\xi}, \tau, \hat{\boldsymbol{u}}) &= -\beta^{-1}\ \psi_2^{(2)} + k_{12}\ \psi_1^{(2)} + \frac{\beta^{-1}}{2\pi}\ p_{22}\ P_2^{(2)}
\end{aligned} \tag{34}$$

If we integrate both sides of each equation over $\hat{\boldsymbol{u}}$ and sum up the equations, we get the following conservation equation:

$$\partial_\tau P_{\text{tot}}^{(0)}(\boldsymbol{\xi}, \tau) + \nabla_\xi \cdot (\boldsymbol{J}_0^{(1)} + \nu\ \boldsymbol{J}_1^{(1)}) = 0, \tag{35}$$

where $P_{\text{tot}}^{(0)} = P_0^{(0)} + P_1^{(0)} + P_2^{(0)}$ is the total zeroth-order density of cells, and $\boldsymbol{J}_i^{(1)} = \int \hat{\boldsymbol{u}}\ \psi_i^{(1)}(\boldsymbol{\xi}, \tau, \hat{\boldsymbol{u}})\ \mathrm{d}\hat{\boldsymbol{u}}$ is the first-order flux of cells in state $i$. This equation can also be reached by appealing to solvability conditions (e.g. [8]). Thus, if we can compute the first-order fluxes and show that they are proportional to spatial gradients of $P_{\text{tot}}^{(0)}$, then we have our diffusion equation.

To do this, we first need to solve the zeroth order equations. At zeroth order in $\epsilon$, there are no derivatives, so we can integrate the equations over all of the dependent variables. This gives a set of algebraic equations for the fraction of time spent in each state at zeroth order, $p_i = \int\int\int \psi_i^{(0)}(\boldsymbol{\xi}, \tau, \hat{\boldsymbol{u}})\ \mathrm{d}\boldsymbol{\xi}\ \mathrm{d}\tau\ \mathrm{d}\hat{\boldsymbol{u}}$:

$$\begin{aligned}
0 &= -k_{01}\ p_0 + k_{10}\ p_1 + \beta^{-1}(p_{10}\ p_1 + p_{20}\ p_2) \\
0 &= -(\beta^{-1}\ p_{10} + k_{10} + k_{12})\ p_1 + k_{01}\ p_0 + \beta^{-1}\ p_{21}\ p_2 \\
0 &= -\beta^{-1}(1 - p_{22})\ p_2 + k_{12}\ p_1.
\end{aligned} \tag{36}$$

Solving these gives the fraction of time spent in each state, as shown in the main text:

$$\begin{aligned}
p_0 = \frac{1}{1+a+b},\ p_1 &= \frac{a}{1+a+b},\ p_2 = \frac{b}{1+a+b}, \\
a &= \frac{k_{01}}{\beta^{-1}\ p_{10} + k_{10} + k_{12}\frac{p_{20}}{p_{20}+p_{21}}}, \\
b &= a\ \frac{k_{12}}{\beta^{-1}(1-p_{22})}
\end{aligned} \tag{37}$$

A further implication of there being no derivatives at zeroth order is that:

$$\psi_i^{(0)}(\boldsymbol{\xi}, \tau, \hat{\boldsymbol{u}}) = p_i \frac{1}{2\pi} P_{\text{tot}}^{(0)}(\boldsymbol{\xi}, \tau); \tag{38}$$

i.e. heading and state are uncorrelated with position and time, or with each other.

Next we turn to the first-order equations. Here, spatial derivatives of zeroth order terms will appear. From Eqn. 35, we are really only interested in the first-order fluxes, $\boldsymbol{J}_i^{(1)}(\boldsymbol{\xi}, \tau)$, for $i \in \{0, 1\}$. To get equations for these, we multiply both sides of the first two equations in Eqns. 32 by $\hat{\boldsymbol{u}}$ and then integrate over $\hat{\boldsymbol{u}}$. The first-order terms in $\epsilon$ are then:

$$\begin{aligned}
\nabla_\xi \cdot \left(\int \hat{\boldsymbol{u}}\ \hat{\boldsymbol{u}}\ \psi_0^{(0)}\ \mathrm{d}\hat{\boldsymbol{u}}\right) &= -\left(\beta^{-1} + k_{01}\right) \boldsymbol{J}_0^{(1)} + k_{10}\ \boldsymbol{J}_1^{(1)} \\
\nu\ \nabla_\xi \cdot \left(\int \hat{\boldsymbol{u}}\ \hat{\boldsymbol{u}}\ \psi_1^{(0)}\ \mathrm{d}\hat{\boldsymbol{u}}\right) &= -\left(\beta^{-1} + k_{10} + k_{12}\right) \boldsymbol{J}_1^{(1)} \\
&\quad + k_{01}\ \boldsymbol{J}_0^{(1)},
\end{aligned} \tag{39}$$

Above, we used $\int \hat{\boldsymbol{u}}\ \mathrm{d}\hat{\boldsymbol{u}} = 0$ to drop all $P_i^{(1)}$ terms. The terms on the left-hand side above can be simplified using Eqn. 38 and the identity $\int \hat{\boldsymbol{u}}\ \hat{\boldsymbol{u}}\ \mathrm{d}\hat{\boldsymbol{u}} = \frac{2\pi}{d}\boldsymbol{I}$ in 2D (e.g. [8]), where $\boldsymbol{I}$ is the identity matrix and $d = 2$:

$$\begin{aligned}
\frac{1}{d}\ p_0\ \nabla_\xi P_{\text{tot}}^{(0)} &= -\left(\beta^{-1} + k_{01}\right) \boldsymbol{J}_0^{(1)} + k_{10}\ \boldsymbol{J}_1^{(1)} \\
\nu\ \frac{1}{d}\ p_1\ \nabla_\xi P_{\text{tot}}^{(0)} &= -\left(\beta^{-1} + k_{10} + k_{12}\right) \boldsymbol{J}_1^{(1)} \\
&\quad + k_{01}\ \boldsymbol{J}_0^{(1)}.
\end{aligned} \tag{40}$$

Solving these, we get the first-order fluxes, which are proportional to spatial gradients of cell densities, as expected:

$$\begin{aligned}
\boldsymbol{J}_0^{(1)}(\boldsymbol{\xi}, \tau) &= -\frac{1}{d}\ \frac{1}{\Lambda_0} \left(p_0 + \nu\ \frac{k_{10}}{\Lambda_1} p_1\right) \nabla_\xi P_{\text{tot}}^{(0)} \\
\boldsymbol{J}_1^{(1)}(\boldsymbol{\xi}, \tau) &= -\nu\ \frac{1}{d}\ \frac{1}{\Lambda_1}\ p_1 \nabla_\xi P_{\text{tot}}^{(0)} + \frac{k_{01}}{\Lambda_1} \boldsymbol{J}_0^{(1)}.
\end{aligned} \tag{41}$$

As in the main text, $\Lambda_1 = \beta^{-1}+k_{10}+k_{12}$ is the decorrelation rate of flux in state 1 and $\Lambda_0 = \beta^{-1}+k_{01}\,(1-k_{10}/\Lambda_1)$ is that in state 0.

Thus, from the prefactor on $-\nabla_\xi P_{\text{tot}}^{(0)}$ in Eqns. 35 and 41, we get the effective diffusion coefficient in the main text:

$$D_{\text{eff}} = \frac{\phi_{\text{void}}}{d}\Bigg(\frac{1}{\Lambda_0}p_0 + \frac{\nu}{\Lambda_0}\;\frac{k_{10}}{\Lambda_1}\;p_1 + \frac{\nu}{\Lambda_1}\;\frac{k_{01}}{\Lambda_0}\left(p_0+\nu\;\frac{k_{10}}{\Lambda_1}\;p_1\right) + \frac{\nu^2}{\Lambda_1}\;p_1\Bigg). \tag{42}$$

Importantly, we have introduced a factor of $\phi_{\text{void}}$ into the diffusion coefficient. As discussed in the main text, the abstracted Markov model erases the obstacles and therefore does not account for the fact that they exclude volume. To reintroduce the effect of excluded volume, we consider a large control volume (or rather, control area) containing many obstacles. Some of the boundary of this control volume intersects obstacles, which do not allow flux through. The fraction of unblocked surface area (or perimeter) is the same as the fraction of a very long line that lies in the void space, which is exactly the void volume fraction. Thus, we expect all fluxes to be proportional to $\phi_{\text{void}}$, and we reintroduce this factor in the diffusion coefficient. This factor is essential for the theoretical expression for the diffusion coefficient to agree with simulations.

## DILUTE OBSTACLE APPROXIMATION

To derive the optimal run length, $\beta^*$, it is useful to study the dilute obstacle regime, in which $\gamma \gg 1$. Since the void percolation threshold in 2D, $\gamma_c^{2D} \sim 1.39$, is larger than 1, the large-$\gamma$ approximation can be accurate for almost the entire range of $\gamma$ that shows diffusive behavior.

Towards deriving a dilute obstacle approximation to the diffusion coefficient, we multiply out all of the products of terms in Eqn. 42. Collecting terms by powers of the run length $\beta$ gives a rational polynomial in $\beta$:

$$D_{\text{eff}} = \frac{\phi_{\text{void}}}{d}\beta\frac{1+A(\gamma)\;\beta+B(\gamma)\;\beta^2}{1+C(\gamma)\;\beta+D(\gamma)\;\beta^2+E(\gamma)\;\beta^3+f(\gamma)\;\beta^4}, \tag{43}$$

where $A(\gamma)$, $B(\gamma)$, ..., $F(\gamma)$ are coefficients of the polynomial, which depend on $\gamma$. These are:

$$\begin{aligned}
A(\gamma) &= \frac{k_{10}\;(1+p_{10})(1-p_{22})+k_{12}\;(p_{20}+p_{10}\;(1-p_{22}))+\nu\;k_{01}\;(p_{10}+\nu)(1-p_{22})}{p_{10}\;(1-p_{22})}\\
B(\gamma) &= \frac{k_{12}^2\;p_{20}+k_{10}^2\;(1-p_{22})+k_{10}\;k_{12}\;(2p_{20}+p_{21})+\nu\;k_{01}\;k_{12}\;p_{20}+2\;\nu\;k_{01}\;k_{10}\;(1-p_{22})+\nu^2\;k_{01}^2\;(1-p_{22})}{p_{10}\;(1-p_{22})}\\
C(\gamma) &= \frac{(k_{01}+k_{10})(1+p_{10})(1-p_{22})+k_{12}\;(p_{20}+p_{10}(1-p_{22}))}{p_{10}\;(1-p_{22})}\\
D(\gamma) &= \frac{k_{01}^2\;(1-p_{22})+(k_{10}+k_{12})(k_{10}(1-p_{22})+k_{12}\;p_{20})+k_{01}(2k_{10}(1-p_{22})+k_{12}\;(1+p_{20}+(1+p_{10})(1-p_{22})))}{p_{10}\;(1-p_{22})}\\
E(\gamma) &= k_{10}\;k_{12}\;\frac{k_{12}(1+p_{20})+(k_{01}+k_{10})(2-p_{22})}{p_{10}\;(1-p_{22})}\\
F(\gamma) &= \frac{k_{01}^2\;k_{12}^2}{p_{10}\;(1-p_{22})},
\end{aligned} \tag{44}$$

Recall that $k_{10} \sim \mathcal{O}(\gamma^0)$, $k_{12} \sim \mathcal{O}(\gamma^{-1})$, and $k_{01} \sim \mathcal{O}(\gamma^{-1})$. Then, anticipating that the optimal run length $\beta^* \sim \gamma^2$, the leading-order $\gamma$ scaling of each term is:

$$\begin{aligned}
A(\gamma)\;\beta^* &\sim \mathcal{O}(\gamma^2)\\
B(\gamma)\;(\beta^*)^2 &\sim \mathcal{O}(\gamma^4)\\
C(\gamma)\;\beta^* &\sim \mathcal{O}(\gamma^2)\\
D(\gamma)\;(\beta^*)^2 &\sim \mathcal{O}(\gamma^4)\\
E(\gamma)\;(\beta^*)^3 &\sim \mathcal{O}(\gamma^4)\\
F(\gamma)\;(\beta^*)^4 &\sim \mathcal{O}(\gamma^4).
\end{aligned} \tag{45}$$

As a result of this scaling, we expect the terms with coefficients $A(\gamma)$ and $C(\gamma)$ to be negligible when $\gamma \gg 1$, i.e. the dilute regime. Therefore, we can neglect them when $\gamma$ is large, as well as the 1's. In fact, the other terms are two factors of $\gamma$ larger than these two terms, so this approximation should be good even when $\gamma$ is not so large.

Keeping terms up to (sub-leading) order $\gamma^3$ in $D_{\text{eff}}$:

$$\begin{aligned}
D_{\text{eff}} &\approx \frac{\phi_{\text{void}}}{d}\beta\frac{B(\gamma)\;\beta^2}{D(\gamma)\;\beta^2+E(\gamma)\;\beta^3+F(\gamma)\;\beta^4},\;\gamma \gg 1\\
&= \frac{\phi_{\text{void}}}{d}\frac{\beta}{D'(\gamma)+E'(\gamma)\;\beta+F'(\gamma)\;\beta^2}.
\end{aligned} \tag{46}$$

The coefficients are:

$$
\begin{aligned}
D'(\gamma) &= \frac{D(\gamma)}{B(\gamma)} \approx 1 + \frac{k_{01}}{k_{10}}\, 2(1-\nu) + \mathcal{O}(\gamma^{-2}) \\
E'(\gamma) &= \frac{E(\gamma)}{B(\gamma)} \approx \frac{k_{01}\ k_{12}}{k_{10}} \frac{2-p_{22}}{1-p_{22}} \left(1 - k_{12} \frac{p_{20} + (1-p_{22})^2}{k_{10}\ (1-p_{22})(2-p_{22})}\right) + \mathcal{O}(\gamma^{-4}) \\
F'(\gamma) &= \frac{F(\gamma)}{B(\gamma)} \approx \left(\frac{k_{01}\ k_{12}}{k_{10}}\right)^2 \frac{1}{1-p_{22}} \left(1 - k_{01}\frac{2\nu}{k_{10}} - k_{12}\frac{p_{20}+1-p_{22}}{k_{10}(1-p_{22})}\right) + \mathcal{O}(\gamma^{-6}).
\end{aligned}
\tag{47}
$$

### Optimal run length $\beta^*$

The expression for $D_{\text{eff}}$ in Eqn. 46 can readily be optimized with respect to $\beta$. Setting the derivative with respect to $\beta$ equal to zero gives an expression for the optimal run length, $\beta^*$:

$$
\begin{aligned}
\beta^* &= \sqrt{\frac{D'(\gamma)}{F'(\gamma)}} \\
&\approx \frac{k_{10}}{k_{01}\ k_{12}} \sqrt{1-p_{22}} \\
&+ \frac{1}{k_{01}} \frac{p_{20}+1-p_{22}}{2\sqrt{1-p_{22}}} + \frac{1}{k_{12}}\sqrt{1-p_{22}} + \mathcal{O}(\gamma^0)
\end{aligned}
\tag{48}
$$

At the optimum, the diffusivity is:

$$
\begin{aligned}
D^*_{\text{eff}} &= \frac{\phi_{\text{void}}}{d} \frac{\beta^*}{2\ D'(\gamma) + E'(\gamma)\beta^*} \\
&= \frac{\phi_{\text{void}}}{d} \frac{\beta^*/D'(\gamma)}{2 + c(\gamma)},
\end{aligned}
\tag{49}
$$

where we define $c(\gamma)$ as:

$$
\begin{aligned}
c(\gamma) &= \frac{E'(\gamma)}{\sqrt{D'(\gamma)F'(\gamma)}} \\
&= \frac{2-p_{22}}{\sqrt{1-p_{22}}} + \frac{k_{12}}{k_{10}} \frac{p_{21}\ p_{22}}{2\ (1-p_{22})^{3/2}} + \mathcal{O}(\gamma^{-2}).
\end{aligned}
\tag{50}
$$

In the main text, we showed the leading-order expressions for $\beta^*$, $D^*_{\text{eff}}$, and $c(\gamma)$—that is, the first term in Eqns. 48 and 50, and Eqn. 49 with $D'(\gamma) \approx 1$.

### Curve collapse

The diffusion coefficients in Eqn. 46 collapse when the run length $\beta$ is rescaled by its optimal value and $D_{\text{eff}}$ is rescaled by its maximum. Defining $\delta = \beta/\beta^*$, we have:

$$
\begin{aligned}
\frac{D_{\text{eff}}}{D^*_{\text{eff}}} &= \frac{2 + c(\gamma)}{\beta^*/D'(\gamma)} \frac{\beta^*/D'(\gamma)\ \delta}{1 + \frac{E'(\gamma)}{D'(\gamma)}\ \beta^*\ \delta + \frac{F'(\gamma)}{D'(\gamma)}\ (\beta^*)^2\ \delta^2} \\
&= \delta \frac{2 + c(\gamma)}{1 + c(\gamma)\ \delta + \delta^2}.
\end{aligned}
\tag{51}
$$

Strictly speaking, the diffusion coefficient still depends on $\gamma$ through $c(\gamma)$, so there is no exact collapse at finite $\gamma$. It only loses this dependence on $\gamma$ when $\gamma \gg 1$ and $c(\gamma)$ becomes approximately constant. However, even for finite $\gamma$, Fig. 3 of the main text shows that the curves—and more importantly, the simulation data—do approximately fall on the large-$\gamma$ limit of the universal curve in Eqn. 51.

We can understand the collapse by considering a different rescaling of the length and time scales in the problem. When $\gamma$ is moderately large compared to 1, the radius of the obstacles, $R$, effectively becomes an irrelevant parameter. Since the problem loses a length scale, it also loses a dimensionless parameter. So instead of needing both $\beta$ and $\gamma$ to parameterize the cell's diffusion coefficient, only a combination of the two parameters is needed. In particular, the only relevant dimensionless parameter is $\delta = \beta/\beta^*$.

Starting from Eqn. 46, we first divide top and bottom by $D'(\gamma)$ and then put units back into the equation:

$$
\frac{D'_{\text{eff}}}{R\ v} \approx \frac{\phi_{\text{void}}}{d} \frac{(L_r/R)/D'(\gamma)}{1 + \frac{E'(\gamma)}{D'(\gamma)}\ (L_r/R) + \frac{F'(\gamma)}{D'(\gamma)}\ (L_r/R)^2}, \tag{52}
$$

where $D'_{\text{eff}}$ is the diffusion coefficient with units, and $L_r$ is the mean run length with units. Then, we note that $F'(\gamma)/D'(\gamma) = (\beta^*)^{-2}$. Therefore, we rescale length by $X = R\ \beta^*$ and define $\delta = L_r/(R\ \beta^*)$:

$$
\begin{aligned}
\frac{D''_{\text{eff}}}{R\ v} \frac{X^2}{T} &= \frac{\phi_{\text{void}}}{d} \frac{\delta/(\sqrt{D'(\gamma)\ F'(\gamma)})}{1 + c(\gamma)\ \delta + \delta^2} \\
D''_{\text{eff}} \frac{R\ \beta^*\ D'(\gamma)}{v\ T} &= \frac{\phi_{\text{void}}}{d} \frac{\delta}{1 + c(\gamma)\ \delta + \delta^2}
\end{aligned}
\tag{53}
$$

where $T$ is a (so far unspecified) time scale, and $D''_{\text{eff}}$ is the dimensionless diffusion coefficient in the new non-dimensionalization, and we have used $\beta^* = D'(\gamma)/F'(\gamma)$.

To complete the new non-dimensionalization, we choose the time scale $T$ to be $T = (R/v)\ \beta^*\ D'(\gamma)$, thus giving a diffusion coefficient with just one dimensionless parameter, $\delta$, as expected:

$$
D''_{\text{eff}} = \frac{\phi_{\text{void}}}{d} \frac{\delta}{1 + c(\gamma)\ \delta + \delta^2} \tag{54}
$$

**Effective hop-trap dynamics**

To understand the physical meaning of this non-dimensionalization, it's useful to consider just the leading order terms in $\gamma$ in the approximations above. This corresponds to a very large $\gamma$ approximation, i.e very dilute obstacles. To leading order, we have:

$$\begin{aligned} D'(\gamma) &= 1 + \mathcal{O}(\gamma^{-1}) \\ E'(\gamma) &= \frac{k_{01}\ k_{12}}{k_{10}} \frac{2-p_{22}}{1-p_{22}} + \mathcal{O}(\gamma^{-3}) \\ F'(\gamma) &= \left(\frac{k_{01}\ k_{12}}{k_{10}}\right)^2 \frac{1}{1-p_{22}} + \mathcal{O}(\gamma^{-5}) \\ \beta^* &= \frac{k_{10}}{k_{01}\ k_{12}} \sqrt{1-p_{22}} + \mathcal{O}(\gamma^{1}) \\ c &= \frac{2-p_{22}}{\sqrt{1-p_{22}}} + \mathcal{O}(\gamma^{-1}) \\ D^*_{\text{eff}} &= \frac{\phi_{\text{void}}}{d} \frac{\beta^*}{2+c}, \end{aligned} \tag{55}$$

and $D_{\text{eff}}$ is still given by Eqn. 46, but with the coefficients above. These are the expressions shown in the main text.

Notice that $\nu$ does not appear in any of the terms above. This indicates that, in this limit, only motion in state 0 contributes to the diffusivity. Indeed, we can take the large-$\gamma$ limit of Eqns. 37 and 42 (treating $\beta$ as order $\gamma^2$). For the fraction of time in each state (Eqn. 37), we get:

$$\begin{aligned} a &\approx \frac{k_{01}}{k_{10}} \sim \mathcal{O}(\gamma^{-1}) \\ b &\approx \frac{k_{01}\ k_{12}}{k_{10}} \frac{1}{\beta^{-1}(1-p_{22})} \sim \mathcal{O}(\gamma^{0}) \\ p_0 &\approx \frac{1}{1+b},\ p_1 \approx 0,\ p_2 \approx \frac{b}{1+b}, \end{aligned} \tag{56}$$

which shows that the fraction of time in state 1, $p_1$, goes to zero like $\sim \gamma^{-1}$, while fraction of time in states 0 and 2, $p_0$ and $p_2$ remain order 1. Furthermore, in the large-$\gamma$ limit, the flux decorrelation rates become:

$$\begin{aligned} \Lambda_1 &= \beta^{-1} + k_{10} + k_{12} \approx k_{10} \\ \Lambda_0 &= \beta^{-1} + k_{01}\ (1 - k_{10}/\Lambda_1) \approx \beta^{-1} + \frac{k_{01}\ k_{12}}{k_{10}}, \end{aligned} \tag{57}$$

and the diffusion coefficient (Eqn. 42) becomes:

$$\begin{aligned} D_{\text{eff}} &= \frac{\phi_{\text{void}}}{d} \frac{1}{\Lambda_0} p_0 + \mathcal{O}(\gamma^0) \\ &= \frac{\phi_{\text{void}}}{d} \frac{1}{\beta^{-1} + \frac{k_{01}\ k_{12}}{k_{10}}} \frac{1}{1 + \frac{k_{01}\ k_{12}}{k_{10}} \frac{1}{\beta^{-1}(1-p_{22})}} + \mathcal{O}(\gamma^0) \\ &= \frac{\phi_{\text{void}}}{d} \frac{1}{\beta^{-1} + \frac{k_{01}\ k_{12}}{k_{10}}} \frac{\beta^{-1}(1-p_{22})}{\beta^{-1}(1-p_{22}) + \frac{k_{01}\ k_{12}}{k_{10}}} + \mathcal{O}(\gamma^0) \\ &= \frac{\phi_{\text{void}}}{d} \frac{1}{\beta^{-1} + k_{\text{trap}}} \frac{k_{\text{esc}}}{k_{\text{esc}} + k_{\text{trap}}} + \mathcal{O}(\gamma^0). \end{aligned} \tag{58}$$

In the third line above, we plugged in $p_0$ (Eqn. 56) and $\Lambda_0$ (Eqn. 57). In the last line, we defined the effective trapping rate (state 0 to state 2 transition) and effective escape rate (state 2 to state 0 transition):

$$\begin{aligned} k_{\text{trap}} &= \frac{k_{01}\ k_{12}}{k_{10}} \sim \mathcal{O}(\gamma^{-2}) \\ k_{\text{esc}} &= \beta^{-1}\ (1-p_{22}). \end{aligned} \tag{59}$$

To complete the comparison with Eqn. 46, note that $\beta^*$ in Eqn. 55 is:

$$\beta^* \approx k_{\text{trap}}^{-1}\ \sqrt{1-p_{22}}. \tag{60}$$

Therefore, Eqn. 58 is:

$$\begin{aligned} D_{\text{eff}} &\approx \frac{\phi_{\text{void}}}{d} \frac{1}{\beta^{-1} + k_{\text{trap}}} \frac{\beta^{-1}(1-p_{22})}{\beta^{-1}(1-p_{22}) + k_{\text{trap}}} \\ &= \frac{\phi_{\text{void}}}{d} \frac{\beta}{1 + k_{\text{trap}}\ \beta} \frac{(1-p_{22})}{(1-p_{22}) + k_{\text{trap}}\ \beta} \\ &= \frac{\phi_{\text{void}}}{d} \frac{\beta^*\ \delta}{1 + k_{\text{trap}}\ \beta^*\ \delta} \frac{(1-p_{22})}{(1-p_{22}) + k_{\text{trap}}\ \beta^*\ \delta} \\ &= \frac{\phi_{\text{void}}}{d} \frac{\beta^*\ \delta}{1 + \sqrt{1-p_{22}}\ \delta} \frac{1}{1 + \frac{1}{\sqrt{1-p_{22}}}\ \delta} \\ &= \frac{\phi_{\text{void}}}{d} \frac{\beta^*\ \delta}{1 + c\ \delta + \delta^2}. \end{aligned} \tag{61}$$

Line 3, we substituted $\beta = \beta^*\ \delta$; line 4 we used Eqn. 60. This is exactly the same as Eqn. 58, to leading order in $\gamma$, with the optimal dimensionless parameter $\delta^* = 1$ and maximum $D^*_{\text{eff}}$ equal to that in Eqn. 55.

With Eqns. 59 and 60, we can better understand the physical meaning of the large-$\gamma$ rescaling of the problem, discussed in the previous subsection. The new length scale $X = R\ \beta^*$ is proportional to the average distance traveled between trapping events, and the new time scale $T = (R/v)\ \beta^*$ is proportional the average time between trapping events. The remaining dimensionless parameter, $\delta = \beta/\beta^*$, is roughly the average run length relative to the average distance between trap events. The parameter $p_{22}$ controls how costly it is to get trapped (i.e. how long it takes to escape), and adjusts these length and time scales so that the maximum diffusion coefficient occurs at $\delta^* = 1$.

## HOP AND TRAP TIME DISTRIBUTIONS

The model in Eqn. 32, with adjustments, can be used to derive "hop" and "trap" time distributions, as measured in experiments [14]. In this model, the hop and trap statistics are determined by the rates of state transitions. Since the model is Markovian, all dwell time distributions consist of sums of exponentials.

In particular, the "hop" state is the sum of the density in states 0 and 1. We can solve the dwell time distribution

in the hop state by first solving the joint survival probability of being state 0 or 1, and then marginalizing (summing) over the two states. A hop is defined as a run that is terminated either by a tumble or a trap event (transition state 2). For a population initially with fractions of cells in state 0 and 1, $\mathbf{p}(t=0) = (p_0(t=0), p_1(t=1))$, the fraction of cells in each state that have not yet tumbled or become trapped at time $t$ follows:

$$\begin{aligned} \frac{\mathrm{d}p_0(t)}{\mathrm{d}t} &= -(\beta^{-1} + k_{01})\ p_0(t) + k_{10}\ p_1(t) \\ \frac{\mathrm{d}p_1(t)}{\mathrm{d}t} &= -(\beta^{-1} + k_{10} + k_{12})\ p_1(t) + k_{01}\ p_0(t) \end{aligned} \tag{62}$$

or

$$\frac{\mathrm{d}\mathbf{p}(t)}{\mathrm{d}t} = -\mathbf{A}\ \mathbf{p}(t). \tag{63}$$

These equations can be solved by finding the eigenvalues $\{\mu_i\}$ and eigenvectors $\{\mathbf{v}_i\}$ of $\mathbf{A}$:

$$\begin{aligned} \mu_\pm &= \beta^{-1} + \frac{1}{2}(k_{01} + k_{10} + k_{12}) \pm \sqrt{k_{01}^2 + 2k_{01}\ (k_{10} - k_{12}) + (k_{10} + k_{12})^2} \\ \mathbf{v}_\pm &\propto \begin{bmatrix} -k_{01} + k_{10} + k_{12} \pm \sqrt{k_{01}^2 + 2k_{01}\ (k_{10} - k_{12}) + (k_{10} + k_{12})^2} \\ 2\ k_{01} \end{bmatrix} \end{aligned} \tag{64}$$

The eigenvalues give the decay rates of the two exponential modes, where $\mu_+$ is the rate of a fast-decaying mode and $\mu_-$ is that of a slower mode. In the dilute obstacle regime, they become:

$$\begin{aligned} \mu_+ &= \beta^{-1} + k_{10} + \mathcal{O}(\gamma^{-1}) \\ \mu_- &= \beta^{-1} + \frac{k_{01}\ k_{12}}{k_{10}} + \mathcal{O}(\gamma^{-3}) \\ &\approx \beta^{-1} + k_{\text{trap}}. \end{aligned} \tag{65}$$

For $\gamma \gg 1$, $\mu_- \ll \mu_+$, so the small decay rate $\mu_-$ captures the effective, long-time hop-trap dynamics. At the other extreme of dense obstacles, $\gamma \ll 1$ (ignoring the fact that $\gamma < 1 < \gamma_c^{2D}$ does not allow diffusive behavior), the decay rates are:

$$\begin{aligned} \mu_+ &= \beta^{-1} + k_{01} + \mathcal{O}(\gamma^0) \\ \mu_- &= \beta^{-1} + k_{12} + \mathcal{O}(\gamma^0), \end{aligned} \tag{66}$$

and thus the hopping time scale is set by the shorter of the tumble rate or the obstacle encounter rate. This is consistent with experimental measurements in an environment where chord lengths were much shorter than the mean run length [14]. There, the hop length distribution is approximately the same as the chord length distribution of the medium. In making this comparison, we assume that the hop length is roughly the same as the hop duration multiplied by the swimming speed.

The trap time distribution in experiments was observed to be a power law with exponent between -2 and -3 [14, 15]. It is possible for a power law with this range of exponents to arise from a mixture of exponential functions whose decay rates vary over orders of magnitude [16, 17]. Technically, every trap in the environment has a different, exponential trap time distribution, where the escape rate depends on the distance between the centers of the two trapping obstacles, $r$.

The probability that a single tumble leads to escape is $1-p_{22}(r)$, where $p_{22}(r)$ is given in Eqn. 28. If the tumble fails to lead to escape, then the cell must wait until the next tumble to try to escape. As discussed earlier in the subsection **Transitions due to tumbles**, the average number of tumbles to escape is $\langle N \rangle = 1/(1 - p_{22}(r))$. Therefore, the mean trap duration, $\tau_{\text{trap}}(r)$, in a trap associated with obstacle spacing $r$ is:

$$\begin{aligned} \tau_{\text{trap}}^{-1}(r) &= \beta^{-1}\ \left(1 - p_{22}(r)\right) / \langle N \rangle \\ &= \beta^{-1}\ \left(1 - p_{22}(r)\right)^2. \end{aligned} \tag{67}$$

The trap time distribution should thus be a mixture of exponentials with decay rates given by the expression above. From Eqn. 28, $p_{22}(r) \in [0, 1/2]$ since $\theta_n(r) \in [0, \pi/2]$. As a result, the ratio of the smallest and largest mean trap durations, among all trap configurations, is 4. That is, the range of mean trap durations varies by a factor of 4. Regardless of the distribution of $r$, this is too small a range of variation to produce a power law over multiple decades of trap duration. Emergence of a power law therefore requires other sources of variation in the mean trap time, such as variations in $\beta$ among individual cells [18–26], or possibly due to steric interactions that were not included in the model here.

## SIMULATION DETAILS

Discrete-time simulations were performed using custom code written in MATLAB (MathWorks, Natick, MA). To accurately capture the cell's dynamics on surfaces and the run length statistics, simulations were

performed using a different non-dimensionalization from that in the main text and the previous sections: length was rescaled by the obstacle radius $R$ as above, but time was rescaled by the mean run duration $\lambda^{-1}$. Units were converted back to those in the main text after the simulation. Time was evolved by Euler integration with a time step of $\Delta t = 1/50$ in these units (i.e. 1/50 of the average run duration).

The cell velocity $\boldsymbol{v}$ was determined by a force-free condition: in free space, the balance between a propulsion force and a drag force makes $\boldsymbol{v}(t) = \hat{\boldsymbol{u}}(t)$, after rescaling the drag coefficient to be 1. When the cell is in contact with an obstacle and pointing towards it, $\hat{\boldsymbol{u}}(t) \cdot \boldsymbol{n}(\boldsymbol{x}_c(t)) < 0$, the normal component of the cell's velocity is zero $\boldsymbol{v}(t) \cdot \boldsymbol{n}(\boldsymbol{x}_c(t))$=0, where $\boldsymbol{n}(\boldsymbol{x}_c(t))$ is the surface normal at the point of contact $\boldsymbol{x}_c$.

The simulations leveraged the fact that obstacles are placed independently of each other to build the environment as the cell explored it. The environment was built in a growing domain of overlapping squares with dimensionless side length $L = \max(10, 10\ \Delta x)$, where $\Delta x$ is the distance the cell travels through free space in one time step. When the cell came within a distance $1 + \Delta x$ of the edge of any square (i.e. 1 obstacle radius plus the distance the cell travels in $\Delta t$), the simulation domain was extended by placing a new square centered at the cell's location. Making this threshold distance larger than the radius of an obstacle ensures that the cell did not reach a location that might be covered by an obstacle that had not yet been placed. Obstacles were then generated in the new square as follows: the number of obstacles placed was sampled from a Poisson distribution with mean $\langle N \rangle = \rho\, L^2 = L^2/(2\gamma)$, and their centers were sampled uniformly at random within the square. Since new squares overlapped with existing ones, any new obstacles whose centers fell inside an existing square were thrown out.

The simulation was initialized by sampling initial locations uniformly at random in the first square until a point in the void space was found. The cell's heading was sampled from a uniform distribution, $\phi \in [0, 2\pi]$.

At initialization, the code checked whether the cell was contained in a closed pore. This was also done after every new set of obstacles was placed for the smallest value of $\gamma$ simulated. If the cell was inside a closed pore, the simulation was ended and restarted with new realizations of the obstacles and initial cell position. There is no way for a cell to swim into a closed pore with fixed obstacles, so it would be nonsensical to simulate those cases. Furthermore, the long-time dynamics in closed pores are guaranteed to not be diffusive, and could bias the mean squared displacement to appear sub-diffusive.

To check whether the cell was in a closed pore, we first sampled points in the void space uniformly at random at number density (number of points per area) $\rho_s = 150\ \rho$, much higher than the density of obstacles. The algorithm went as follows. Starting from the cell's location, search within a circular neighborhood for nearby points. Using the distribution of nearest neighbor distances between points (Eqn. 7), the radius $r_s$ of this circle was chosen so that the probability of not finding a neighbor was $10^{-8}$. This radius was still small $r \ll 1$ because because $\rho_s \gg \rho$ was large. Points found in the search were added to a running list, excluding repeat points. From each new point added to the list, this process was repeated until a point along the edge of the simulation domain was found, indicating that the cell is not trapped in a closed pore, or until no new neighboring points were found, indicating that the cell was trapped in a closed pore.

To generate tumbles, in each time step, a uniform random number $r \in [0, 1]$ was sampled. If $r < \Delta t$, the cell tumbled in that time step; otherwise, it continued running. This scheme samples run durations that are exponentially distributed with mean duration 1. When the cell tumbled, its heading was sampled uniformly at random from $\phi \in [0, 2\pi]$, and its speed was set to zero for that time step. In the time steps when the cell did not tumble, the code solved the dynamics of cell motion, encounters with obstacles, and motion along obstacles piece-wise analytically with sub-$\Delta t$ resolution. The total simulation time was $T = 2000$ (in units of average run durations), and $N_{sim} = 750$ simulations were run per parameter set, each with a different realization of the environment.

$D_{\text{eff}}$ was estimated from simulations by computing the mean square displacement (MSD) of each trajectory (Methods) and fitting a line to the average MSD. MSD curves were fit for times $t \geq 500$ to exclude initial transients, either due to the time it took cells with large $\beta$ to tumble, or due to the time it took cells with small $\beta$ to diffuse a distance comparable to the size of an obstacle. Dividing the slope of the fit line by $2\ d$ gave $D_{\text{eff}}$. For each parameter pair $(\beta, \gamma)$, error bars on $D_{\text{eff}}$ were computed by bootstrapping: $N_{sim}$ simulation trajectories were randomly drawn with replacement, and $D_{\text{eff}}$ for the sample was computed as above; this process was repeated 100 times, and the error bar was taken to be the standard deviation of the 100 replicates.

Analytical calculations were aided by Mathematica (Wolfram).

* hmattingly@flatironinstitute.org

[1] W. Strieder and R. Aris, *Variational Methods Applied to Problems of Diffusion and Reaction*, edited by B. D. Coleman, Springer Tracts in Natural Philosophy, Vol. 24 (Springer, Berlin, Heidelberg, 1973).

[2] S. Torquato and B. Lu, Chord-length distribution function for two-phase random media, Physical Review E **47**, 2950 (1993).

[3] B. Lu and S. Torquato, Lineal-path function for ran-

dom heterogeneous materials, Physical Review A **45**, 922 (1992).

[4] B. Lu and S. Torquato, Chord-length and free-path distribution functions for many-body systems, The Journal of Chemical Physics **98**, 6472 (1993).

[5] C. Yang, *Diffusion of Run-and-Tumble Microswimmers in porous media*, Ph.D. thesis, UC San Diego (2020).

[6] D. Saintillan, Dispersion of run-and-tumble microswimmers through disordered media (2023), arXiv:2308.04538 [cond-mat, physics:physics].

[7] B. Ezhilan, R. Alonso-Matilla, and D. Saintillan, On the distribution and swim pressure of run-and-tumble particles in confinement, Journal of Fluid Mechanics **781**, R4 (2015).

[8] A. Celani and M. Vergassola, Bacterial strategies for chemotaxis response, Proceedings of the National Academy of Sciences **107**, 1391 (2010).

[9] F. Sagues and W. Horsthemke, Diffusive transport in spatially periodic hydrodynamic flows, Physical Review A **34**, 4136 (1986).

[10] P. McCarty and W. Horsthemke, Effective diffusion coefficient for steady two-dimensional convective flow, Physical Review A **37**, 2112 (1988).

[11] R. Erban and H. G. Othmer, From Individual to Collective Behavior in Bacterial Chemotaxis, SIAM Journal on Applied Mathematics **65**, 361 (2004).

[12] C. Xue and H. G. Othmer, Multiscale Models of Taxis-Driven Patterning in Bacterial Populations, SIAM Journal on Applied Mathematics **70**, 133 (2009).

[13] A. Bensoussan, J.-L. Lions, and G. Papanicolaou, *Asymptotic analysis for periodic structures* (American Mathematical Society, Providence, R.I, 2011).

[14] T. Bhattacharjee and S. S. Datta, Bacterial hopping and trapping in porous media, Nature Communications **10**, 2075 (2019).

[15] T. Bhattacharjee and S. S. Datta, Confinement and activity regulate bacterial motion in porous media, Soft Matter **15**, 9920 (2019).

[16] Y. Tu and G. Grinstein, How White Noise Generates Power-Law Switching in Bacterial Flagellar Motors, Physical Review Letters **94**, 208101 (2005).

[17] A. C. Costa and M. Vergassola, Fluctuating landscapes and heavy tails in animal behavior (2023), arXiv:2301.01111 [cond-mat, physics:physics].

[18] J. L. Spudich and D. E. Koshland, Non-genetic individuality: chance in the single cell, Nature **262**, 467 (1976).

[19] E. Korobkova, T. Emonet, J. M. G. Vilar, T. S. Shimizu, and P. Cluzel, From molecular noise to behavioural variability in a single bacterium, Nature **428**, 574 (2004).

[20] H. Park, W. Pontius, C. C. Guet, J. F. Marko, T. Emonet, and P. Cluzel, Interdependence of behavioural variability and response to small stimuli in bacteria, Nature **468**, 819 (2010).

[21] J.-B. Masson, G. Voisinne, J. Wong-Ng, A. Celani, and M. Vergassola, Noninvasive inference of the molecular chemotactic response using bacterial trajectories, Proceedings of the National Academy of Sciences **109**, 1802 (2012).

[22] Y. S. Dufour, S. Gillet, N. W. Frankel, D. B. Weibel, and T. Emonet, Direct Correlation between Motile Behavior and Protein Abundance in Single Cells, PLOS Computational Biology **12**, e1005041 (2016).

[23] A. J. Waite, N. W. Frankel, Y. S. Dufour, J. F. Johnston, J. Long, and T. Emonet, Non-genetic diversity modulates population performance, Molecular Systems Biology **12**, 895 (2016).

[24] A. J. Waite, N. W. Frankel, and T. Emonet, Behavioral Variability and Phenotypic Diversity in Bacterial Chemotaxis, Annual Review of Biophysics **47**, 595 (2018).

[25] H. H. Mattingly, K. Kamino, B. B. Machta, and T. Emonet, Escherichia coli chemotaxis is information limited, Nature Physics , 1 (2021).

[26] H. H. Mattingly and T. Emonet, Collective behavior and nongenetic inheritance allow bacterial populations to adapt to changing environments, Proceedings of the National Academy of Sciences **119**, e2117377119 (2022).
